# Supplementary material for: Algorithmic Prompt-Augmentation for Efficient LLM-Based Heuristic Design for A* Search
Source: arXiv:2601.19622 source file (2026-01-27)
Supplement: Supplementary file 1 [file appendix.tex]

\section{Appendix}
\label{appendix}

\begin{figure}[h!tbp]
\centering
\begin{framed}
\begin{justify}
\begin{minipage}{1\textwidth}
\tiny
\textcolor{black}{
Act as a professional algorithm designer. Design a heuristic to guide the tree search. \\
}
\par
\par
\textcolor{black}{
I have 5 existing algorithms with their codes as follows: 
\newline
No. 1 algorithm and the corresponding code are: 
\newline
\{thoughts\}
\newline
\{program code\}
\newline
No. 2 algorithm and the corresponding code are: ... \\
}
\par
\textcolor{black}{
First, describe your new algorithm and main steps in one sentence.
The description must be inside a brace.
Next, implement it in Python as a function named \texttt{score\_state}. 
This function should accept 1 input(s): \texttt{'state'}. 
The function should return 1 output(s): \texttt{'score'}. 
\texttt{'state'} is the configuration of lanes after a move. 
The output named \texttt{'score'} is the score for the warehouse state.   \\
}

\textcolor{black}{
Note that 'state' is a two levels nested list with integers in the second level sublist.  \texttt{'score'} must be an integer or float. Avoid utilizing the random component, and it is crucial to maintain self-consistency.
Do not use libraries. Do not use 'while' loops. Do not give additional explanations. Don't create additional methods and please avoid nesting methods. 
}
\end{minipage}
\end{justify}
\end{framed}
\caption{UPMP: E1 strategy prompt template for baseline case.}
\label{fig: p1_prompt_upmp_eoh}
\end{figure}

\begin{figure}[h!tbp]
\centering
\begin{framed}
\begin{justify}
\begin{minipage}{1\textwidth}
\tiny
\textcolor{black}{
Act as a professional algorithm designer. Design a heuristic to guide the tree search. \\
}
\par
\textcolor{mydarkgreen}{
\textbf{ALGORITHMIC CONTEXT}\\
}
\par
\textcolor{black}{
I have 5 existing algorithms with their codes as follows: 
\newline
No. 1 algorithm and the corresponding code are: 
\newline
\{thoughts\}
\newline
\{program code\}
\newline
No. 2 algorithm and the corresponding code are: ... \\
}
\par
\textcolor{black}{
First, describe your new algorithm and main steps in one sentence.
The description must be inside a brace.
Next, implement it in Python as a function named \texttt{score\_state}. 
This function should accept 1 input(s): \texttt{'state'}. 
The function should return 1 output(s): \texttt{'score'}. 
\texttt{'state'} is the configuration of lanes after a move. 
The output named \texttt{'score'} is the score for the warehouse state.   \\
}

\textcolor{black}{
Note that 'state' is a two levels nested list with integers in the second level sublist.  \texttt{'score'} must be an integer or float. Avoid utilizing the random component, and it is crucial to maintain self-consistency.
Do not use libraries. Do not use 'while' loops. Do not give additional explanations. Don't create additional methods and please avoid nesting methods. 
}
\end{minipage}
\end{justify}
\end{framed}
\caption{UPMP: E1 strategy prompt template in A-CEoH.}
\label{fig: p1_prompt_upmp_aceoh}
\end{figure}

\begin{figure}[h!tbp]
\centering
\begin{framed}
\begin{justify}
\begin{minipage}{1\textwidth}
\tiny
\textcolor{black}{
Act as a professional algorithm designer. Design a heuristic to guide the tree search. \\
}
\par
\textcolor{red}{
\textbf{ADDITIONAL PROBLEM CONTEXT}\\
}
\par
\textcolor{black}{
I have 5 existing algorithms with their codes as follows: 
\newline
No. 1 algorithm and the corresponding code are: 
\newline
\{thoughts\}
\newline
\{program code\}
\newline
No. 2 algorithm and the corresponding code are: ... \\
}
\par
\textcolor{black}{
First, understand the provided problem description, input, and output examples. 
Then extract the main constraints of the problem.
Second, think about how these constraints affect the requested heuristic. 
Third, describe your new algorithm and main steps in one sentence. The description must be inside a brace. 
Next, implement it in Python as a function named \texttt{score\_state}. 
This function should accept 1 input(s): \texttt{'state'}. 
The function should return 1 output(s): \texttt{'score'}. 
\texttt{'state'} is the configuration of lanes after a move. 
The output named \texttt{'score'} is the score for the warehouse state.   \\
}

\textcolor{black}{
Note that 'state' is a two levels nested list with integers in the second level sublist.  \texttt{'score'} must be an integer or float. Avoid utilizing the random component, and it is crucial to maintain self-consistency.
Do not use libraries. Do not use 'while' loops. Do not give additional explanations. Don't create additional methods and please avoid nesting methods. 
}
\end{minipage}
\end{justify}
\end{framed}
\caption{UPMP: E1 strategy prompt template in P-CEoH.}
\label{fig: p1_prompt_upmp_pceoh}
\end{figure}

\begin{figure}[h!tbp]
\centering
\begin{framed}
\begin{justify}
\begin{minipage}{1\textwidth}
\tiny
\textcolor{black}{
Act as a professional algorithm designer. Design a heuristic to guide the tree search. \\
}
\par
\textcolor{mydarkgreen}{ALGORITHMIC CONTEXT HERE}
\par
\textcolor{red}{
\textbf{ADDITIONAL PROBLEM CONTEXT}\\
}
\par
\textcolor{black}{
I have 5 existing algorithms with their codes as follows: 
\newline
No. 1 algorithm and the corresponding code are: 
\newline
\{thoughts\}
\newline
\{program code\}
\newline
No. 2 algorithm and the corresponding code are: ... \\
}
\par
\textcolor{black}{
Please help me create a new algorithm that has a totally different form from the given ones. 
Please help me create a new algorithm that enriches the given algorithms with the new ideas provided. 
First, understand the provided problem description, input, and output examples. Then extract the main constraints of the problem.
Second, think about how these constraints affect the requested heuristic.
Third, identify the common backbone idea in the provided algorithms.
Fourth, based on the backbone ideas, describe your new algorithm in one sentence. The description must be inside a brace.
Next, implement it in Python as a function named \texttt{score\_state}. 
This function should accept 1 input(s): \texttt{'state'}. 
The function should return 1 output(s): \texttt{'score'}. 
\texttt{'state'} is a list of 2D grids representing the puzzle after a move. 
The output named \texttt{'score'} is the score for the puzzle state.  \\
}

\textcolor{black}{
Note that 'state' is a two levels nested list with integers in the second level sublist.   \texttt{'score'}  must be an integer or float. Avoid utilizing the random component, and it is crucial to maintain self-consistency.
Do not use libraries. Do not use 'while' loops. Do not give additional explanations. Don't create additional methods and please avoid nesting methods. 
}
\end{minipage}
\end{justify}
\end{framed}
\caption{E1 strategy prompt template for the UPMP.}
\label{fig: p1_prompt_upmp}
\end{figure}

\begin{figure}[h!tbp]
\centering
\begin{framed}
\begin{justify}
\begin{minipage}{1\textwidth}
\tiny

\textcolor{red}{
'state' is represented by a two levels deep nested list.
The second level list represents a row of the puzzle as a list of integers.
The first list index (index 0) is the top row of the puzzle.
The highest list index is the bottom row of the puzzle.
A 1 represents the tile numbered 1.
A 20 represents the tile numbered 20.
A 0 represents the empty slot.
Each state has exactly one 0 (empty slot) somewhere in the puzzle.
Only one tile can move into the empty space at any given time.
Each integer represents a tile with its number.
This heuristic should work for puzzles of any size, like 10x10 shown below.
\\
\\
Goal configuration example:\\}
\textcolor{red}{
\[
\begin{bmatrix}
1 & 2 & 3 & 4 & 5 & 6 & 7 & 8 & 9 & 10 \\
11 & 12 & 13 & 14 & 15 & 16 & 17 & 18 & 19 & 20 \\
21 & 22 & 23 & 24 & 25 & 26 & 27 & 28 & 29 & 30 \\
31 & 32 & 33 & 34 & 35 & 36 & 37 & 38 & 39 & 40 \\
41 & 42 & 43 & 44 & 45 & 46 & 47 & 48 & 49 & 50 \\
51 & 52 & 53 & 54 & 55 & 56 & 57 & 58 & 59 & 60 \\
61 & 62 & 63 & 64 & 65 & 66 & 67 & 68 & 69 & 70 \\
71 & 72 & 73 & 74 & 75 & 76 & 77 & 78 & 79 & 80 \\
81 & 82 & 83 & 84 & 85 & 86 & 87 & 88 & 89 & 90 \\
91 & 92 & 93 & 94 & 95 & 96 & 97 & 98 & 99 & 0
\end{bmatrix}
\]}
\textcolor{red}{
First example for \texttt{'state'}:\\
\[
\begin{bmatrix}
1 & 13 & 2 & 14 & 5 & 6 & 7 & 8 & 9 & 10 \\
21 & 11 & 4 & 3 & 15 & 16 & 17 & 18 & 19 & 20 \\
12 & 22 & 23 & 24 & 25 & 26 & 27 & 28 & 29 & 30 \\
32 & 52 & 33 & 53 & 34 & 36 & 37 & 38 & 39 & 40 \\
42 & 41 & 43 & 44 & 35 & 45 & 46 & 48 & 49 & 50 \\
61 & 64 & 31 & 63 & 55 & 56 & 47 & 58 & 59 & 60 \\
62 & 72 & 51 & 54 & 75 & 65 & 0 & 68 & 69 & 70 \\
71 & 82 & 73 & 74 & 77 & 67 & 57 & 78 & 79 & 80 \\
81 & 83 & 84 & 85 & 66 & 76 & 97 & 87 & 88 & 90 \\
91 & 92 & 93 & 94 & 95 & 86 & 96 & 98 & 89 & 99
\end{bmatrix}
\]}
\textcolor{red}{
Second example for \texttt{'state'}:\\
\[
\begin{bmatrix}
1 & 2 & 3 & 4 & 5 & 6 & 7 & 8 & 9 & 10 \\
11 & 12 & 13 & 14 & 15 & 16 & 17 & 18 & 19 & 20 \\
21 & 22 & 23 & 24 & 36 & 25 & 27 & 28 & 29 & 30 \\
31 & 42 & 32 & 33 & 34 & 26 & 37 & 39 & 49 & 40 \\
41 & 52 & 43 & 44 & 35 & 46 & 47 & 38 & 50 & 60 \\
61 & 51 & 53 & 54 & 45 & 56 & 57 & 48 & 80 & 59 \\
71 & 62 & 63 & 64 & 0 & 55 & 66 & 58 & 68 & 78 \\
81 & 72 & 73 & 74 & 65 & 75 & 67 & 90 & 69 & 70 \\
91 & 83 & 93 & 84 & 76 & 86 & 77 & 87 & 79 & 99 \\
92 & 82 & 94 & 95 & 85 & 96 & 97 & 88 & 98 & 89
\end{bmatrix}
\]
}
\textcolor{red}{
First example for \texttt{'score'}: 6\\
Second example for \texttt{'score'}: 0.5
}
\end{minipage}
\end{justify}
\end{framed}
\caption{Additional problem context the SPP.}
\label{fig: pceoh_SPP}
\end{figure}

\begin{figure}[h!tbp]
\centering
\begin{framed}
\begin{justify}
\begin{minipage}{1\textwidth}
\tiny

\textcolor{red}{
'state' is represented by a two levels deep nested list. The second level list represents a lane of unit loads as a list of integers. The first list index (index 0) is the outermost slot in the lane. The highest list index is the innermost slot in the lane. Lanes are accessed from the first index to the highest index. Each integer represents a unit load and its priority class. Unit load of the same priority class are equal. A 1 represents the highest priority class. A 5 represents the lowest priority class. A 3 represents a priority class lower than 1 but higher than 5. A 4 represents a priority class lower than 3 but higher than 5. A 0 represents an empty slot. Each lane must have all 0s (empty slots) grouped at the start or have no 0s at all, ensuring that if any non-zero elements appear in a lane, all subsequent slots must also be non-zero. }
\par
\textcolor{red}{
Therefore, impossible configurations are: [1, 1, 0, 0] or [2,0,2], while possible configurations are: [0, 0, 1, 2] or [1, 2, 3, 3]. 
}
\par
\textcolor{red}{
Examples for blocking unit loads: In the lane [0, 4, 1] the 4 blocks access to 1. 
In the lane [3, 3, 2] the two 3s block access to the 2. 
In the lane [0, 5, 1, 5, 2] the two 5s block access to the 2 and 1. 
In the lane [0, 4, 4, 3] the two 4s block access to the 3. 
}
\par
\textcolor{red}{
First example for 'state': 
}
\textcolor{red}{
\[
\begin{bmatrix}
0 & 2 & 3 \\
0 & 5 & 5 \\
5 & 1 & 1
\end{bmatrix}
\]
}
\textcolor{red}{
Second example for 'state': 
}
\textcolor{red}{
\[
\begin{bmatrix}
2 & 2 & 3 & 5 \\
0 & 3 & 5 & 4\\
0 & 0 & 2 & 2 \\
\end{bmatrix}
\]
}
\\
\textcolor{red}{
First example for 'score': 6.
Second example for 'score': 0.5
}
\end{minipage}
\end{justify}
\end{framed}
\caption{Additional problem context the UPMP.}
\label{fig: pceoh_SPP}
\end{figure}

\begin{figure}[htbp]
\centering
\begin{minipage}{1\textwidth}
\tiny
\begin{lstlisting}[language=Python, label={lst:astar_core}]
def astar_multibay_premarshalling(heuristics, warehouse):
    open_list = []
    visited = set()
    evaluated_nodes = 0

    root = WarehouseNode(warehouse, g=0, heuristic_fn=heuristics.score_state)
    heapq.heappush(open_list, (root.f, 0, evaluated_nodes, root))
    visited.add(root.serialize())
    start_time = time.time()

    while open_list:
        current_time = time.time()
        if (current_time - start_time > TIMEOUT_SECONDS
                or evaluated_nodes > MAX_EVALUATED_NODES):
            return return_result(False)

        _, _, _, current_node = heapq.heappop(open_list)

        if current_node.is_goal():
            return return_result(True)

        for neighbor in current_node.get_neighbors(heuristics.score_state):
            if neighbor.serialize() in visited:
                continue
            evaluated_nodes += 1
            visited.add(neighbor.serialize())
            move_cost = neighbor.state.ap_distance[neighbor.move[0], neighbor.move[1]]
            heapq.heappush(open_list, (neighbor.f, move_cost, evaluated_nodes, neighbor))


def is_goal(self):
    for stack in self.to_list():
        for i in range(len(stack) - 1):
            if stack[i] > stack[i + 1]:
                return False
    return True

def get_neighbors(self, heuristic_fn):
    lanes = self.state.virtual_lanes
    load_indices = [i for i, lane in enumerate(lanes) if np.any(lane.stacks != 0)]
    slot_indices = [i for i, lane in enumerate(lanes) if np.any(lane.stacks == 0)]

    neighbors = []
    for from_idx in load_indices:
        for to_idx in slot_indices:
            if from_idx == to_idx:
                continue
            wh_neighbor = copy.copy(self.state)
            new_lanes = list(lanes)

            new_lane_from, moved_load = lanes[from_idx].remove_load()
            new_lane_to = lanes[to_idx].add_load(moved_load)
            new_lanes[from_idx] = new_lane_from
            new_lanes[to_idx] = new_lane_to
            wh_neighbor.virtual_lanes = new_lanes

            neighbor_node = WarehouseNode(wh_neighbor, g=self.g + 1, heuristic_fn=heuristic_fn, 
            parent=self, move=(from_idx, to_idx))
            neighbors.append(neighbor_node)

    return neighbors

def reconstruct_path(node):
    path = []
    while node.parent is not None:
        path.append((node.move, node.state))
        node = node.parent
    return list(reversed(path))
    
def get_objective_value(self):
    if not self.is_goal():
        return MAX_NUMBER_OF_MOVES
    return len(self.reconstruct_path(self))
    
\end{lstlisting}
\end{minipage}
\caption{Algorithmic context example for the UPMP.}
\label{fig:astar_algorithmic_context}
\end{figure}

\begin{figure}[htbp]
\centering
\begin{minipage}{1\textwidth}
\tiny
\begin{lstlisting}[language=Python, label={lst:astar_core}]
def astar_puzzle_core(heuristics, start_puzzle):
    open_list = []
    visited = set()
    evaluated_nodes = 0
    counter = itertools.count()

    root = PuzzleNode(start_puzzle, g=0, heuristic_fn=heuristics.score_state)
    heapq.heappush(open_list, (root.f, next(counter), root))
    visited.add(root.serialize())
    start = time.monotonic()

    while open_list:
        # Timeout / node cap check
        if ((time.monotonic() - start) > TIMEOUT_SECONDS or 
            evaluated_nodes > MAX_EVALUATED_NODES):
            return return_result(False)

        _, _, current = heapq.heappop(open_list)

        if current.is_goal():
            return return_result(True)

        for neighbor in current.get_neighbors(heuristics.score_state):
            state = neighbor.serialize()
            if state in visited:
                continue
            evaluated_nodes += 1
            visited.add(state)
            heapq.heappush(open_list, (neighbor.f, next(counter), neighbor))

def is_goal(self):
    flat = [num for row in self.puzzle for num in row]
    return flat == list(range(1, self.N * self.N)) + [0]

def get_neighbors(self, heuristic_fn):
    neighbors = []
    r, c = self.find_blank()
    directions = {(-1, 0): 'U', (1, 0): 'D', (0, -1): 'L', (0, 1): 'R'}
    for (dr, dc), move in directions.items():
        nr, nc = r + dr, c + dc
        if 0 <= nr < self.N and 0 <= nc < self.N:
            new_puzzle = deepcopy(self.puzzle)
            new_puzzle[r][c], new_puzzle[nr][nc] = new_puzzle[nr][nc], new_puzzle[r][c]
            neighbors.append(PuzzleNode(new_puzzle, self.g + 1, heuristic_fn, parent=self, move=move))
    return neighbors

def reconstruct_path(node):
    path = []
    while node.parent is not None:
        path.append((node.move, node.puzzle))
        node = node.parent
    return list(reversed(path))
    
def get_objective_value(self):
    if not self.is_goal():
        return MAX_MOVES
    return len(self.reconstruct_path(self))
\end{lstlisting}
\end{minipage}
\caption{Algorithmic context example for the SPP.}
\label{fig:astar_algorithmic_context}
\end{figure}
